# Supplementary material for: Towards Explaining Uncertainty Estimates in Point Cloud Registration
Source: arXiv:2412.20612 source file (2024-12-29)
Supplement: Supplementary file 1 [file appendix.tex]

\appendix

% Although the perturbation is the same on all sequences, the effect seems to be most prominent in \textit{Apartment}, shown from the larger ranges in all three dimensions.

\clearpage % ends the current page and creates a new one
\newgeometry{top=1.5cm}
\begin{figure}[htbp]
    \centering
    \begin{subfigure}[b]{0.47\textwidth}
        \includegraphics[width=\linewidth]{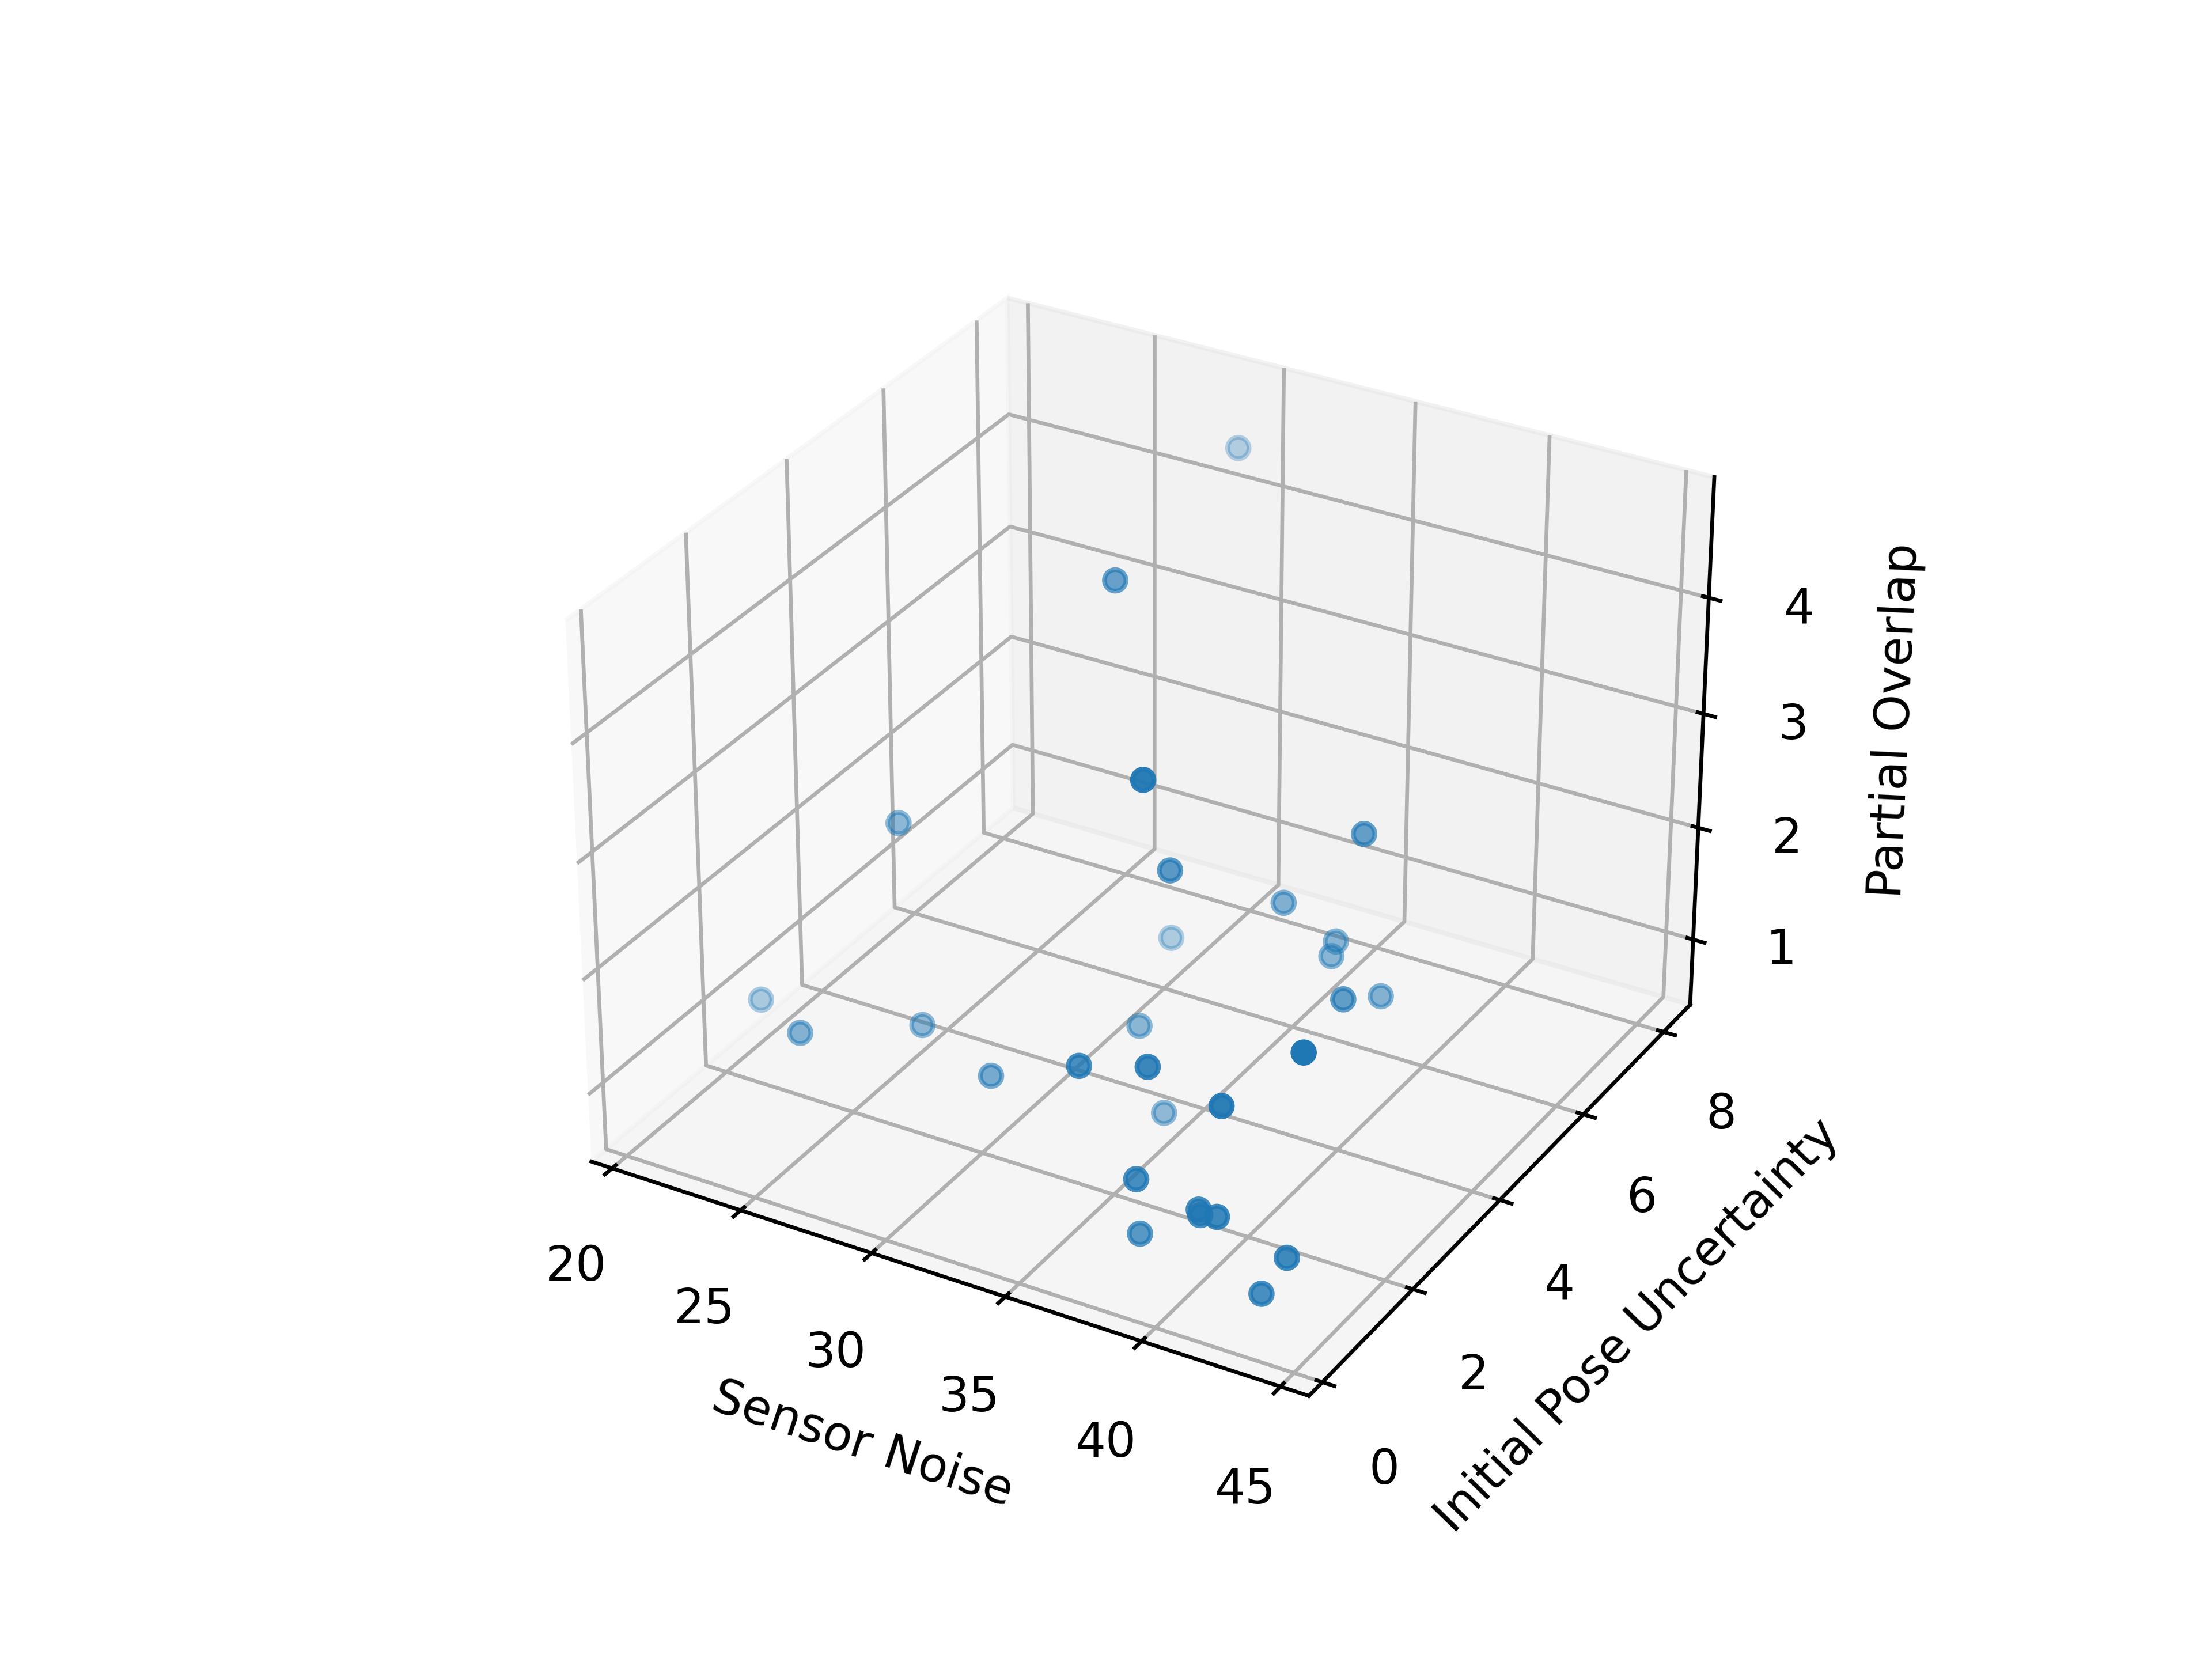}
        \caption{Apartment}
    \end{subfigure}
    \hfill
    \begin{subfigure}[b]{0.47\textwidth}
        \includegraphics[width=\linewidth]{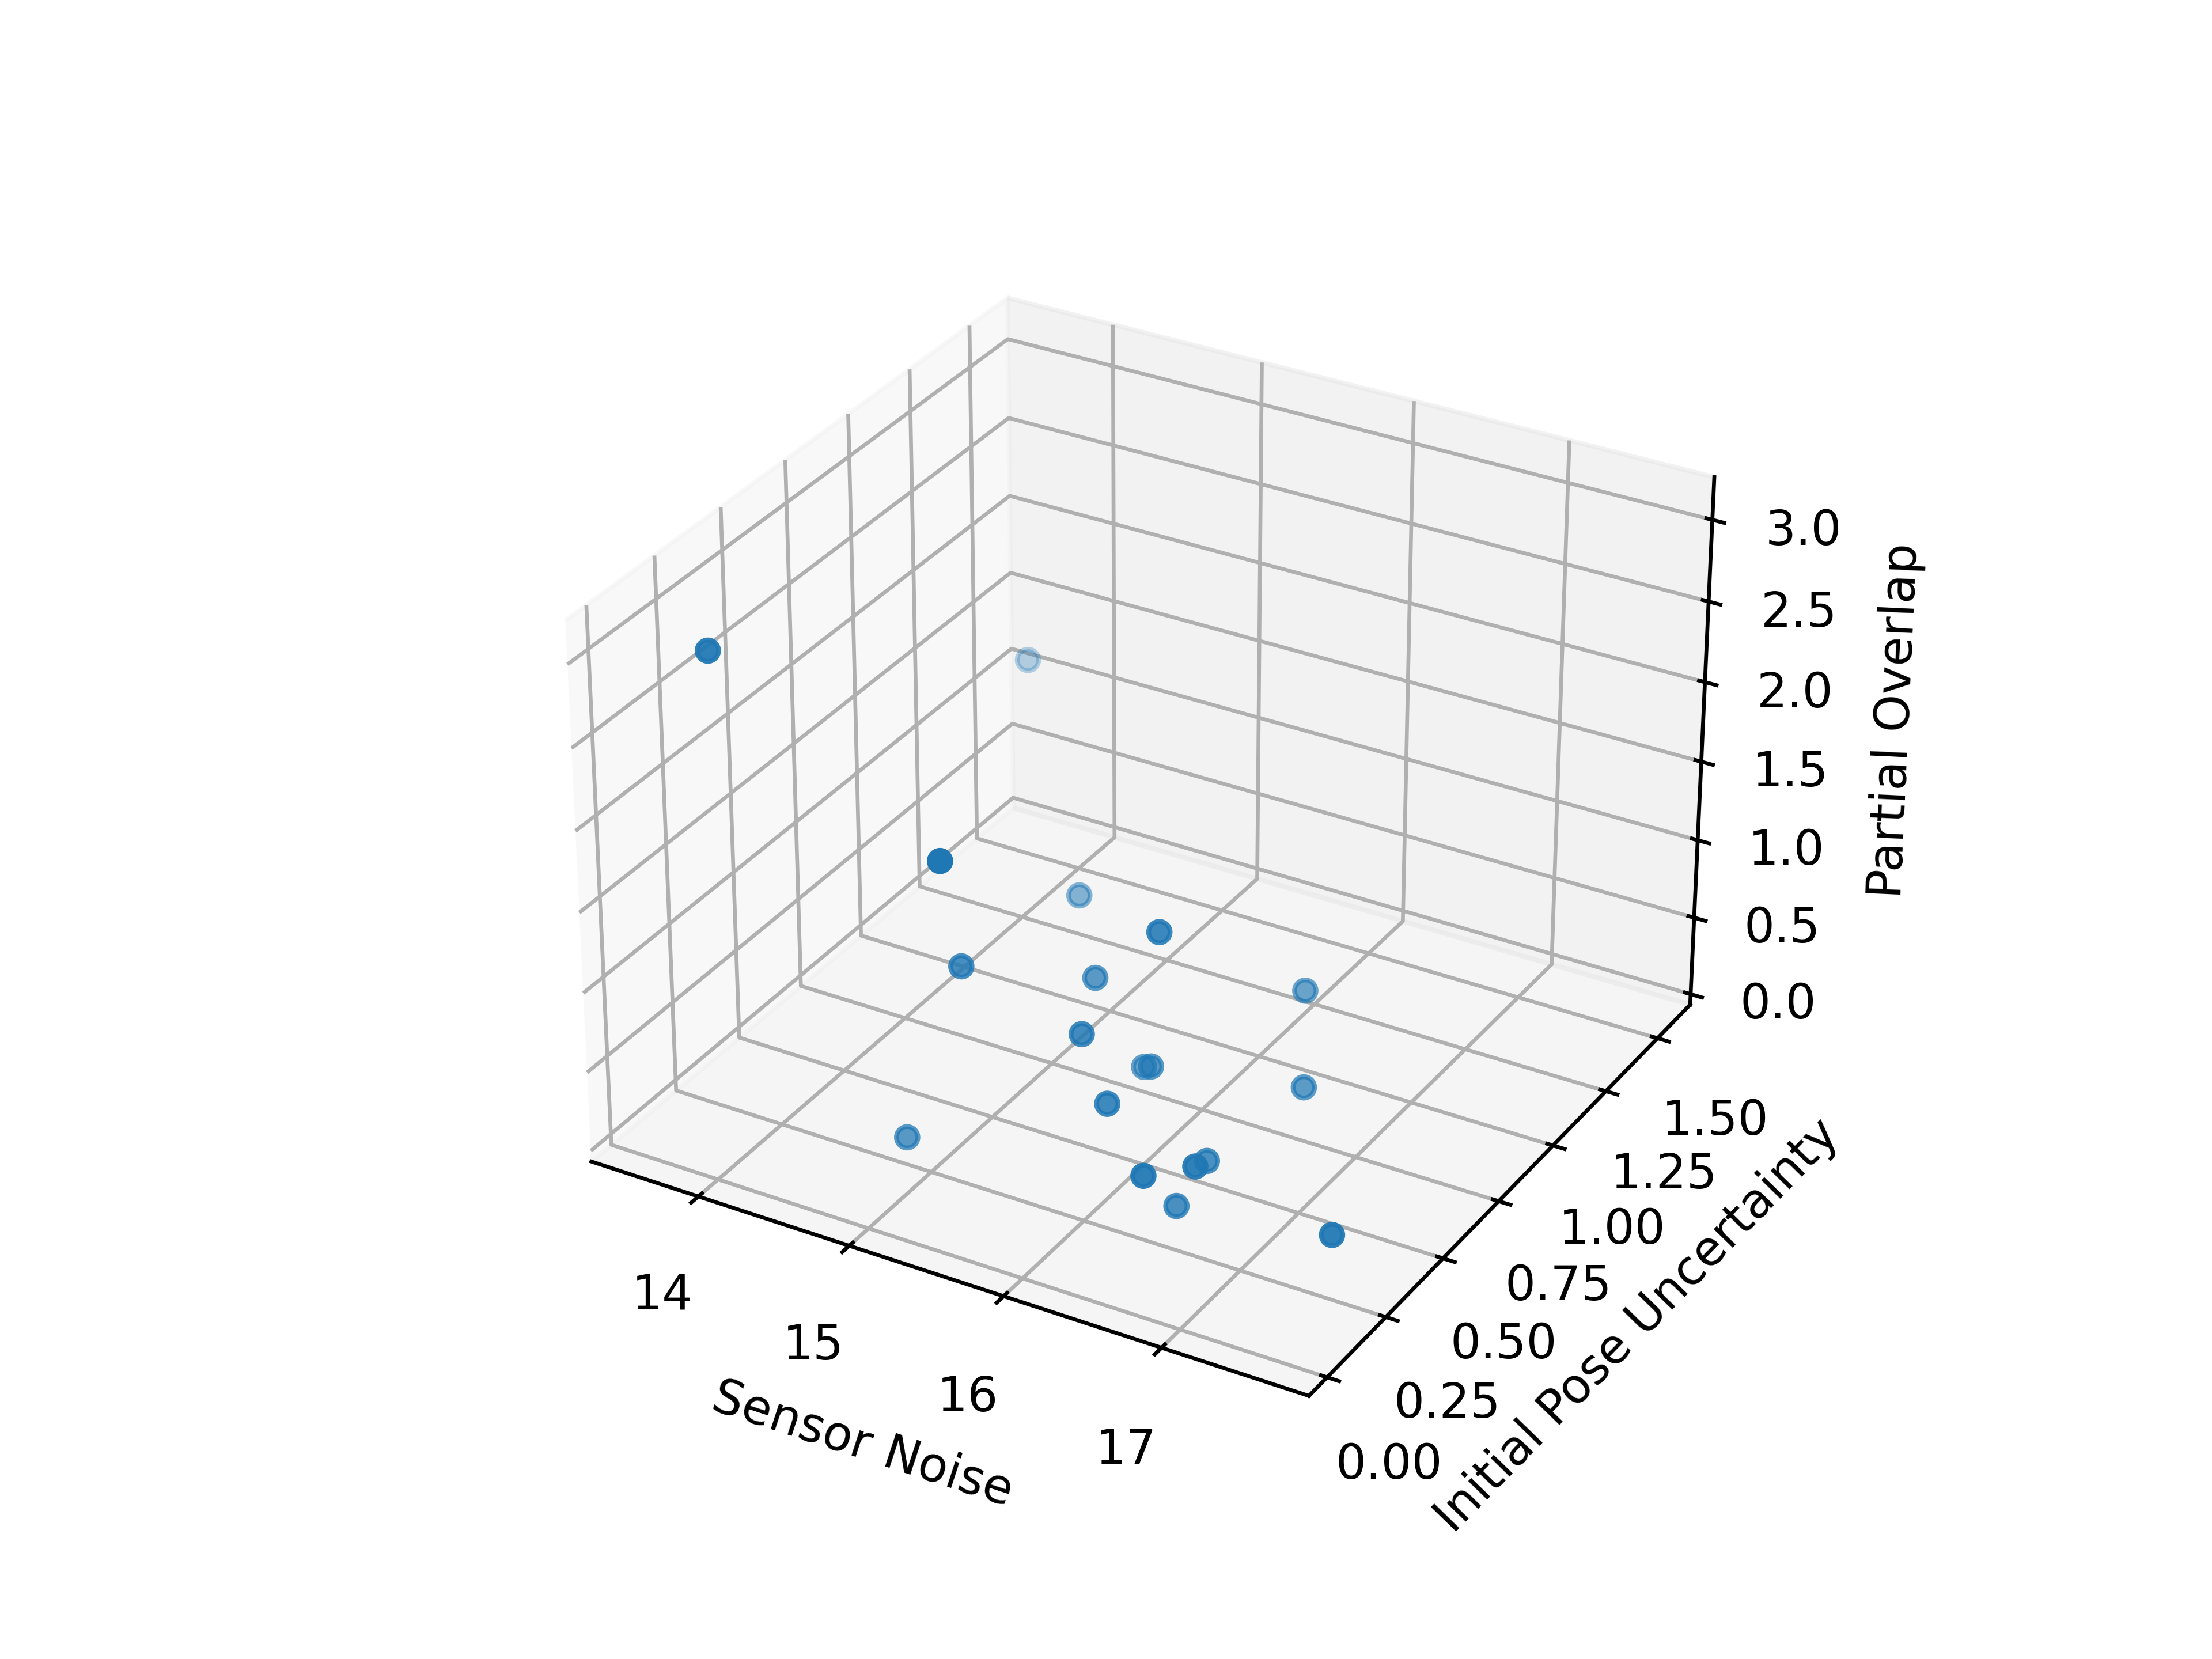}
        \caption{ETH}
    \end{subfigure}
    \begin{subfigure}[b]{0.47\textwidth}
        \includegraphics[width=\linewidth]{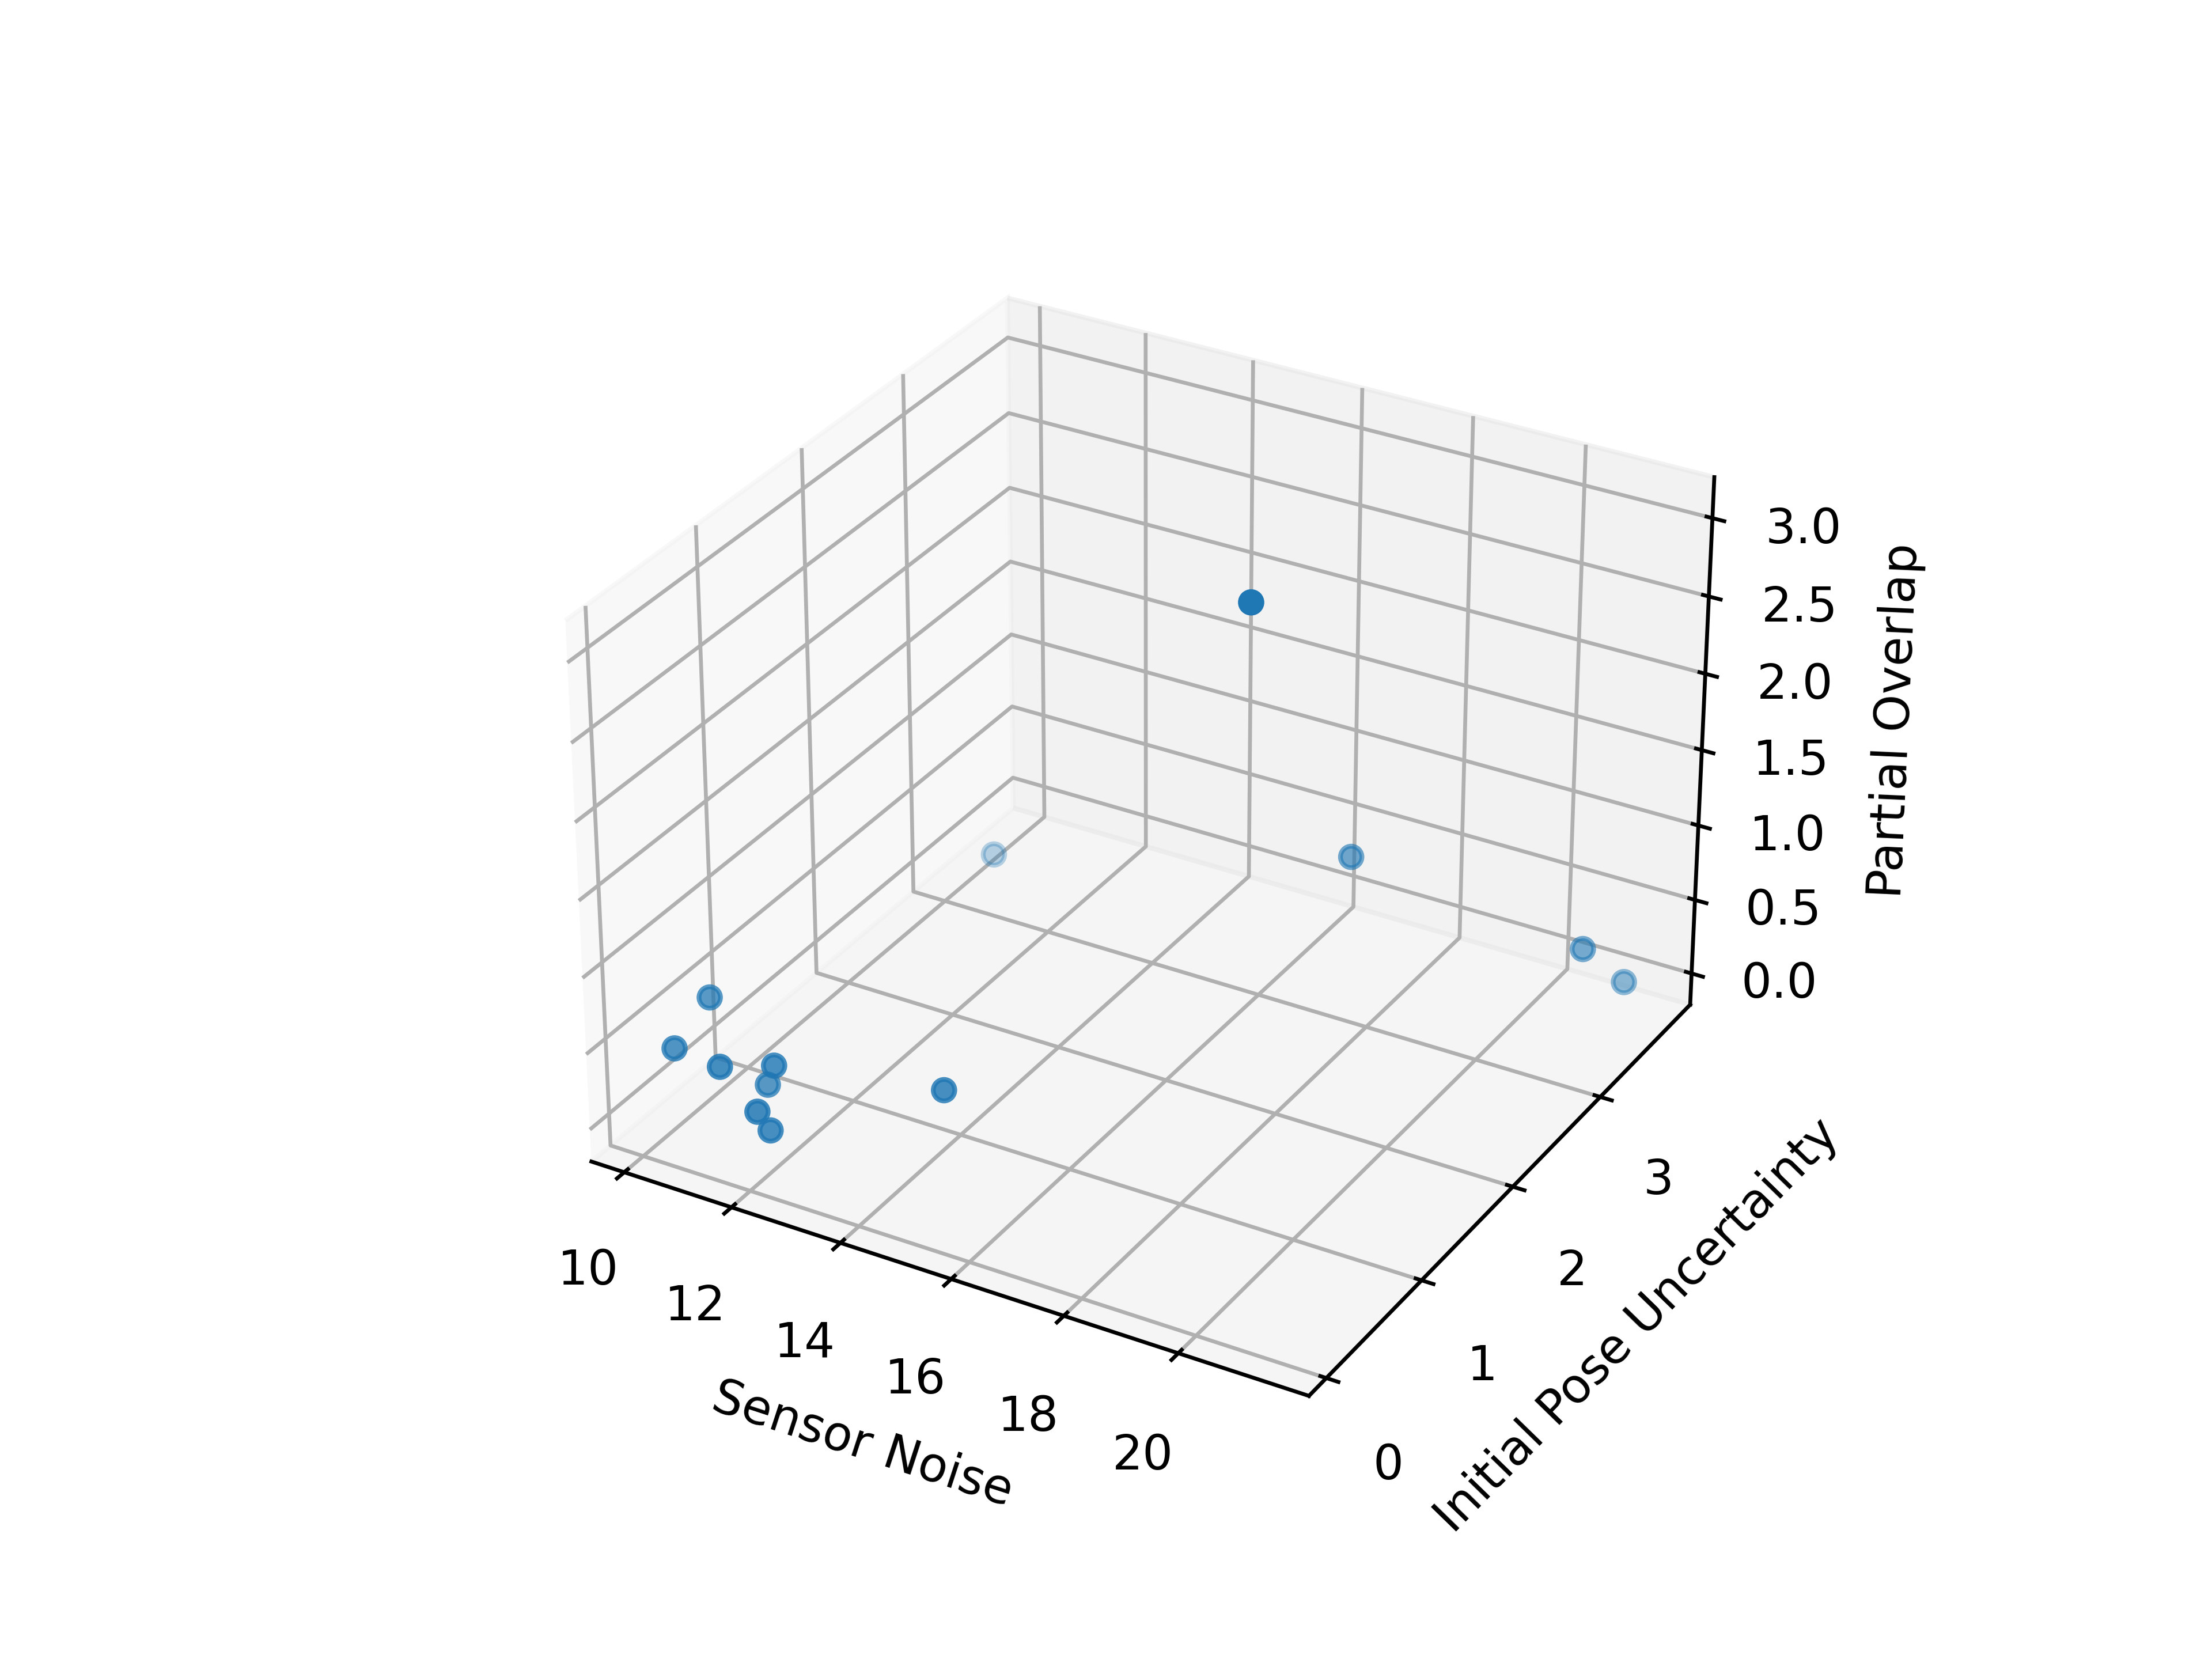}
        \caption{Stair}
    \end{subfigure}
    \hfill
    \begin{subfigure}[b]{0.47\textwidth}
        \includegraphics[width=\linewidth]{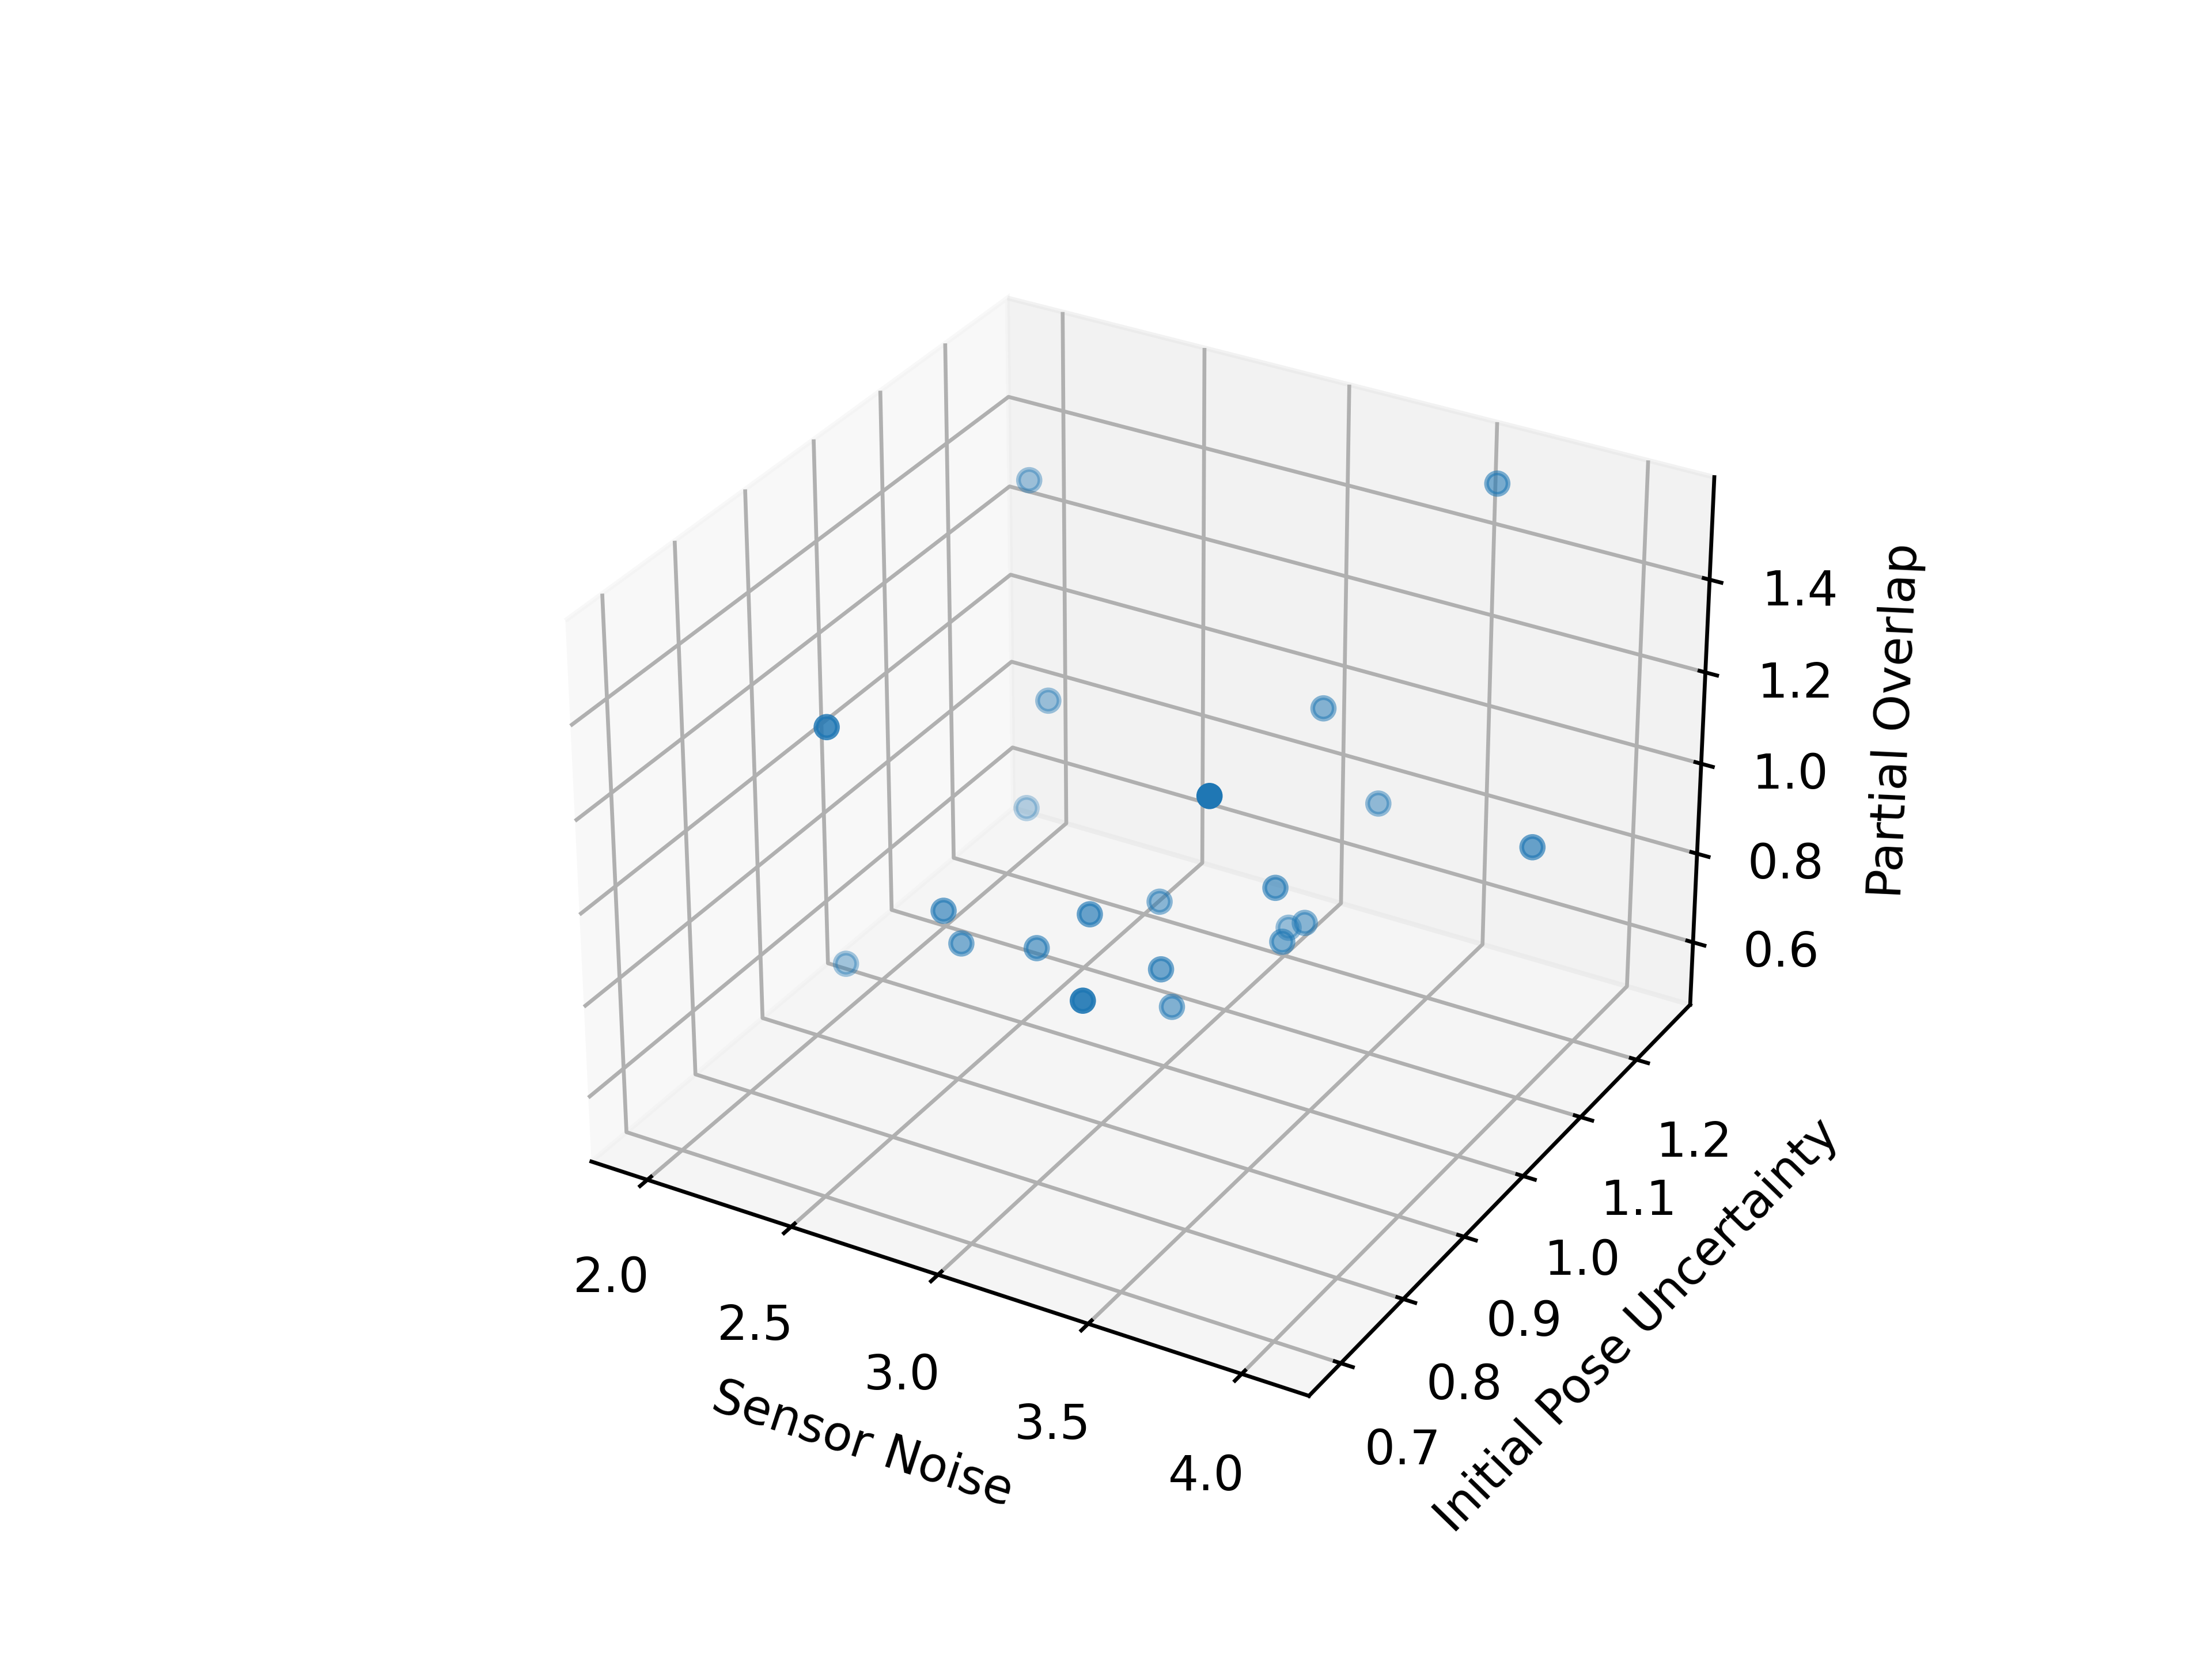}
        \caption{Mountain}
    \end{subfigure}
    \begin{subfigure}[b]{0.47\textwidth}
        \includegraphics[width=\linewidth]{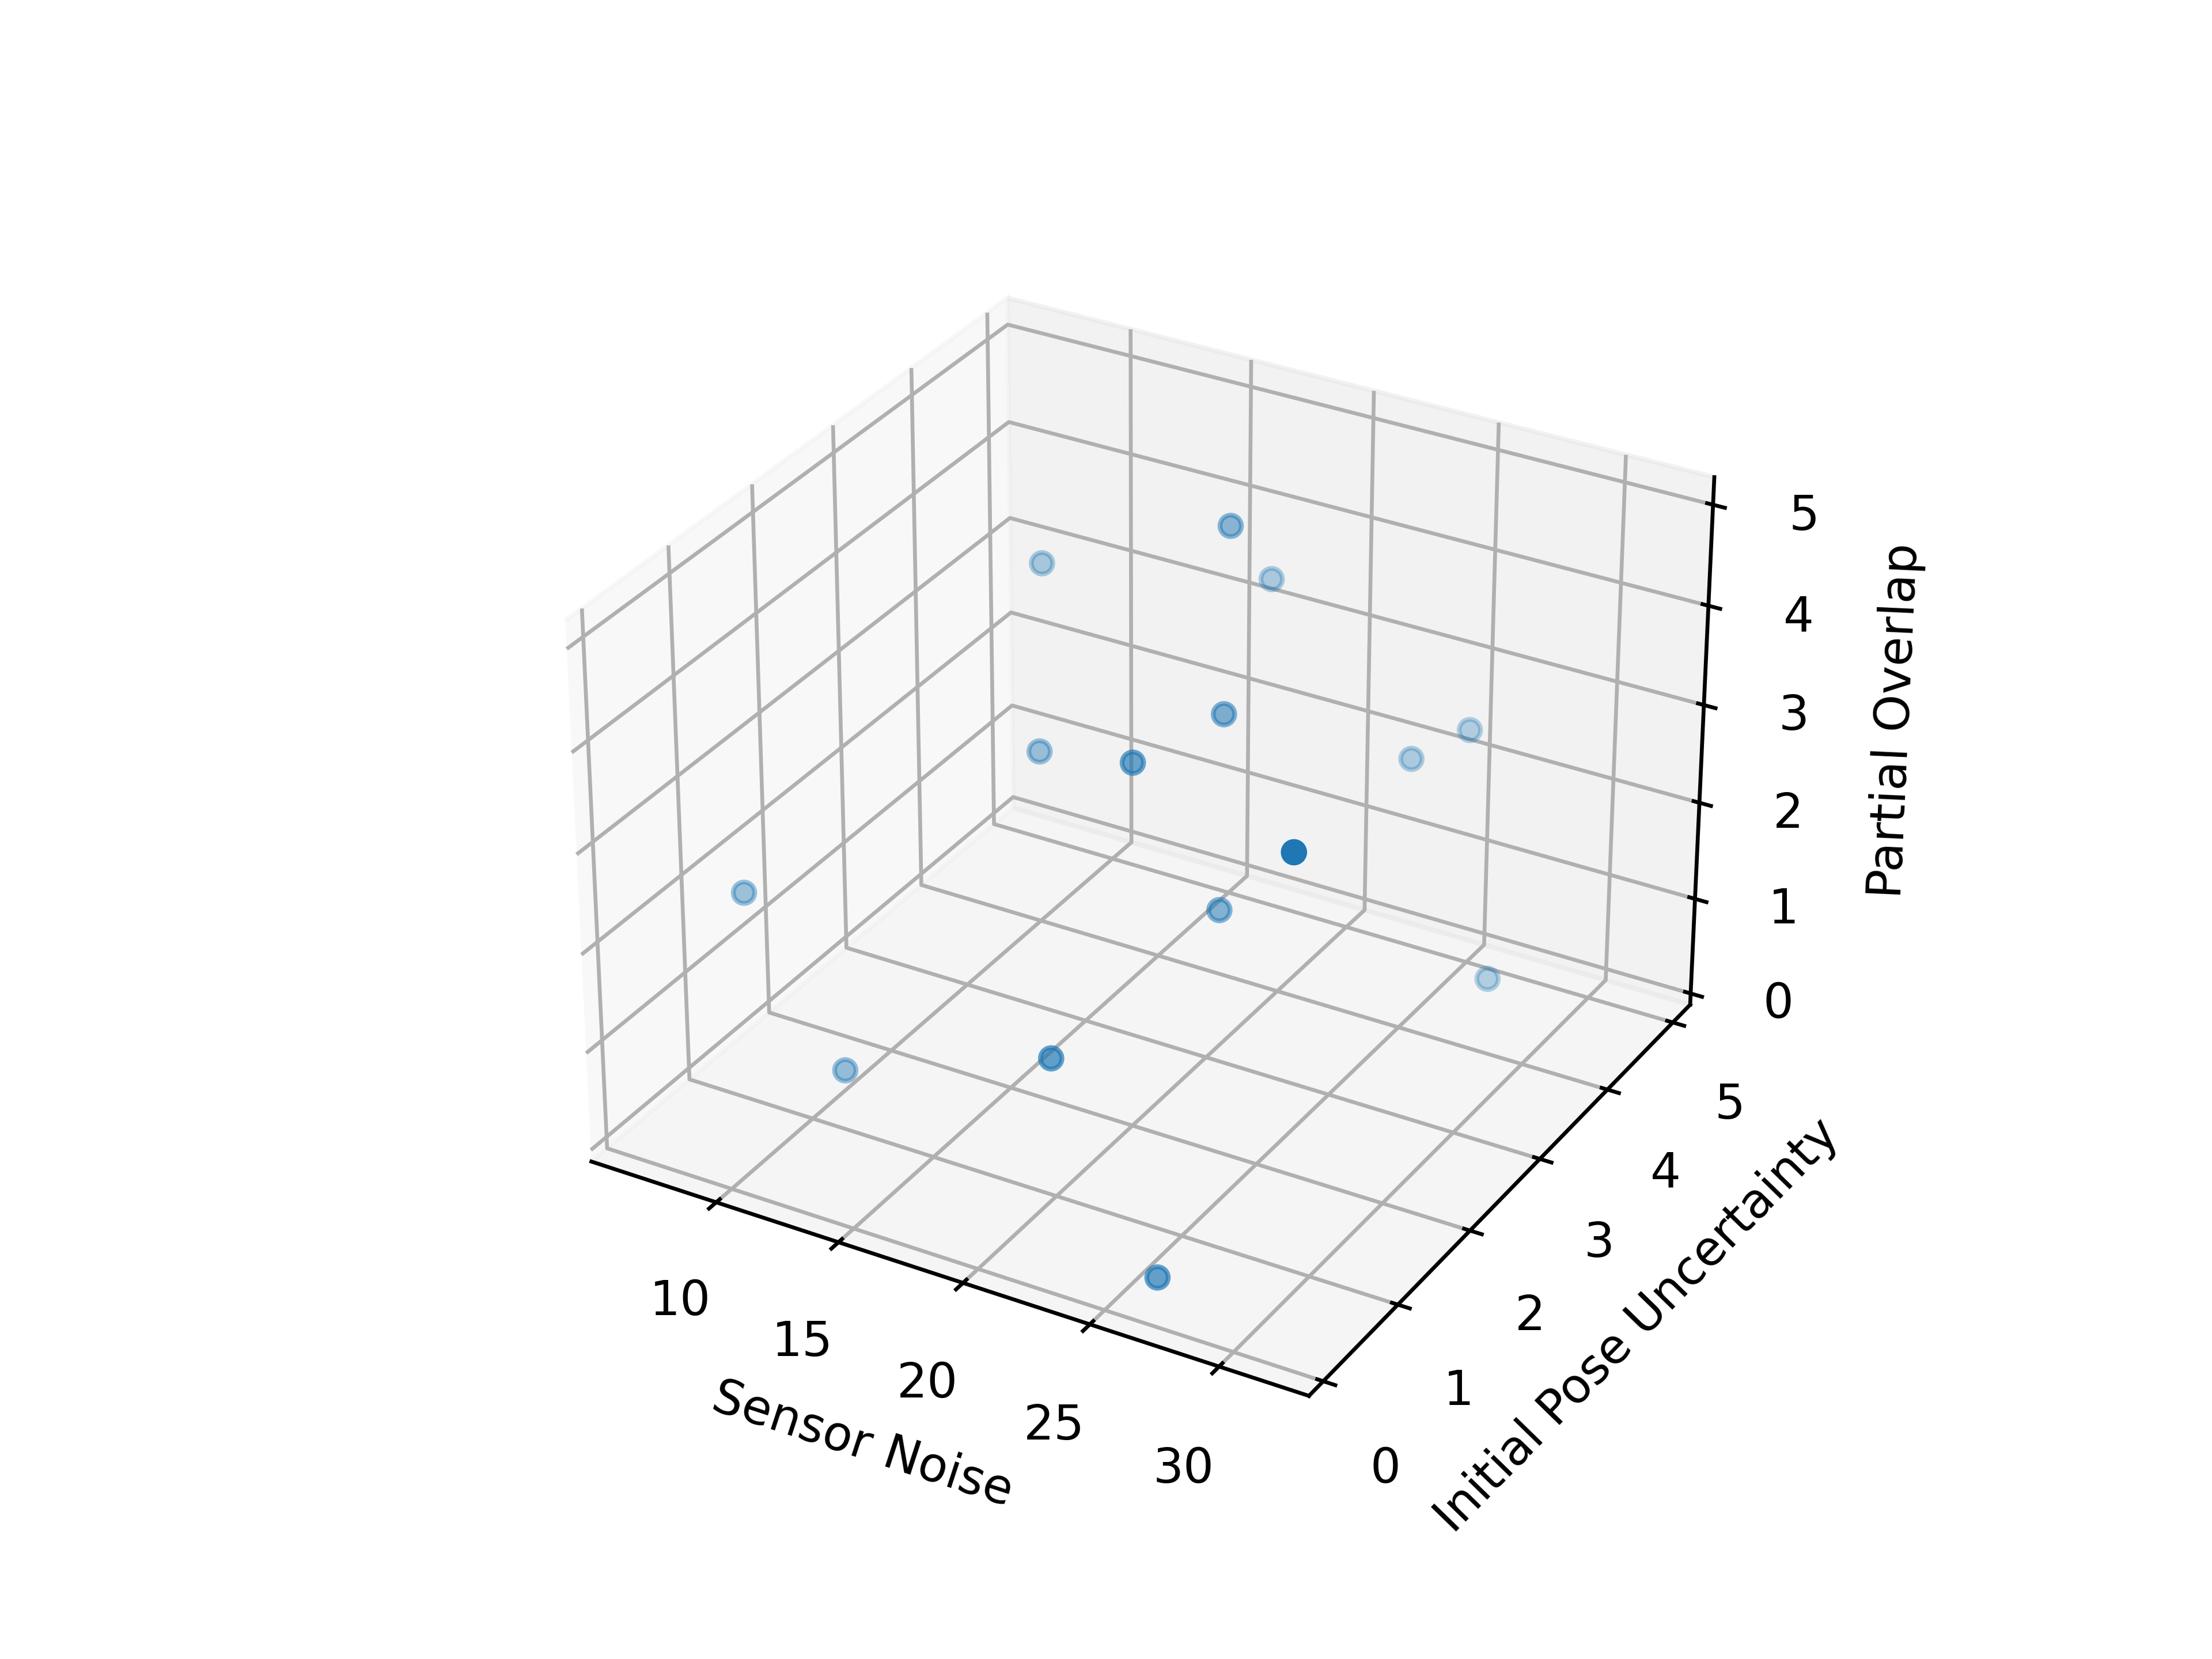}
        \caption{Gazebo Summer}
    \end{subfigure}
    \hfill
    \begin{subfigure}[b]{0.47\textwidth}
        \includegraphics[width=\linewidth]{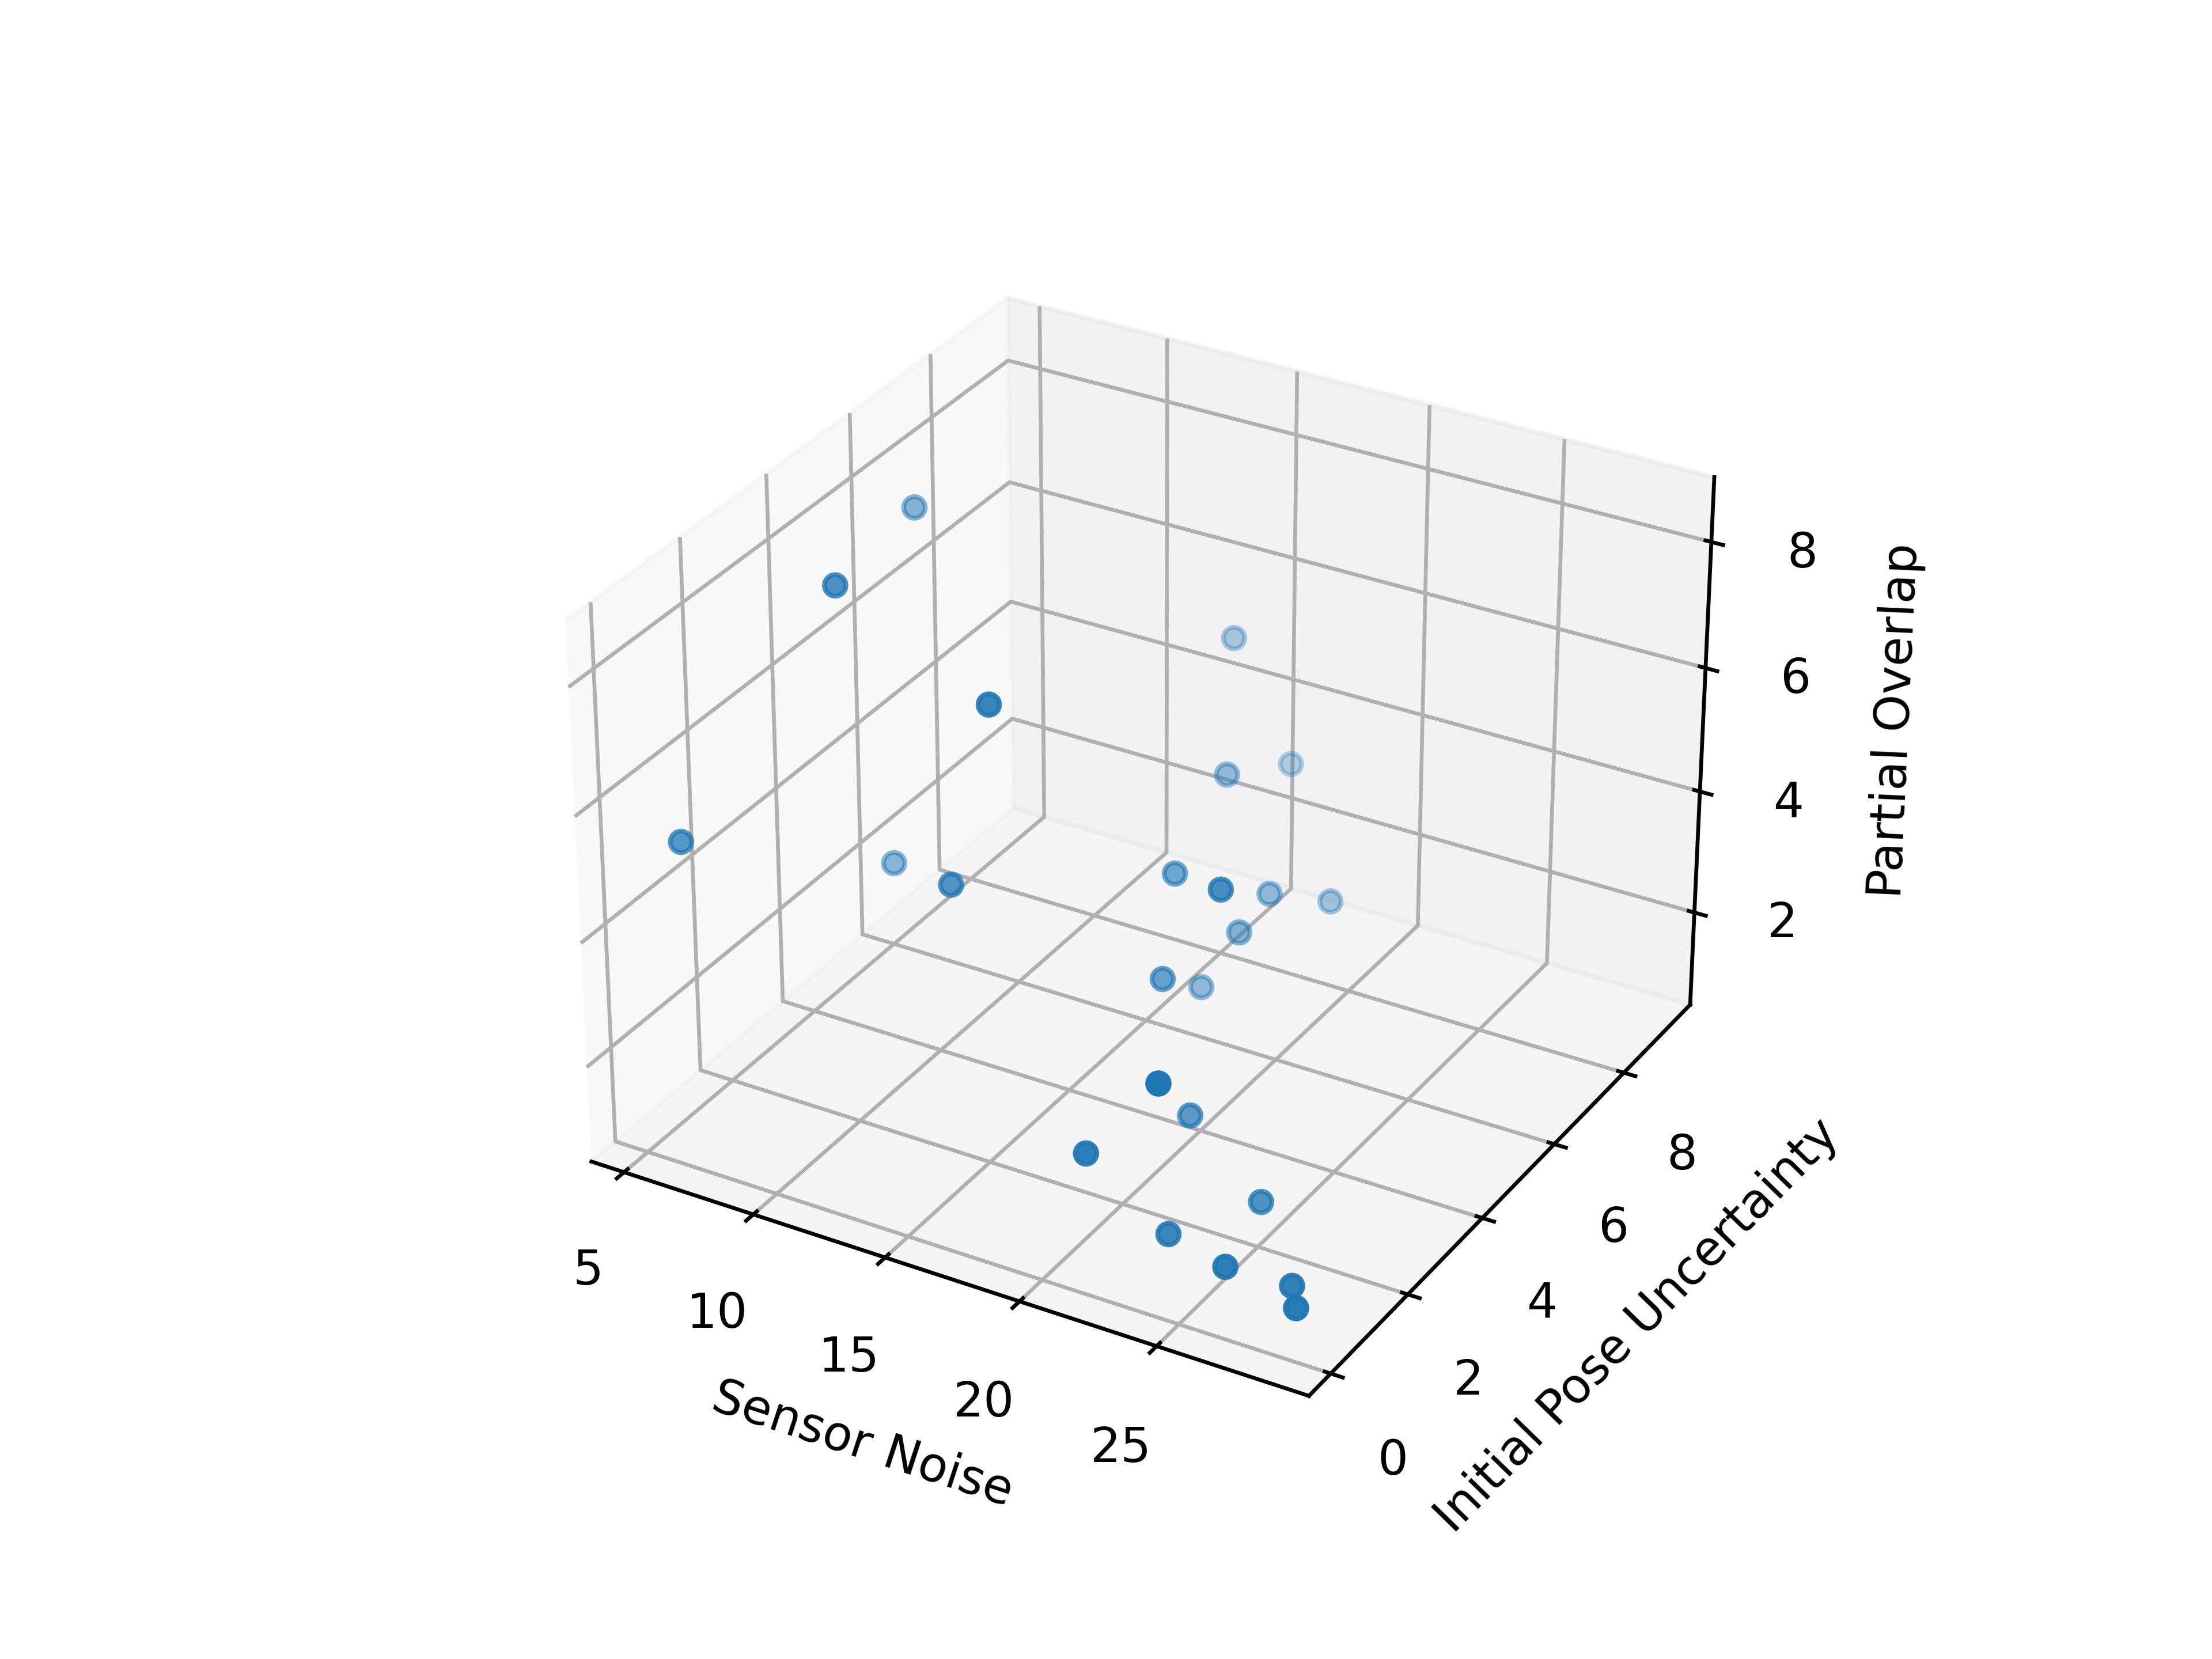}
        \caption{Gazebo Winter}
    \end{subfigure}
    \begin{subfigure}[b]{0.47\textwidth}
        \includegraphics[width=\linewidth]{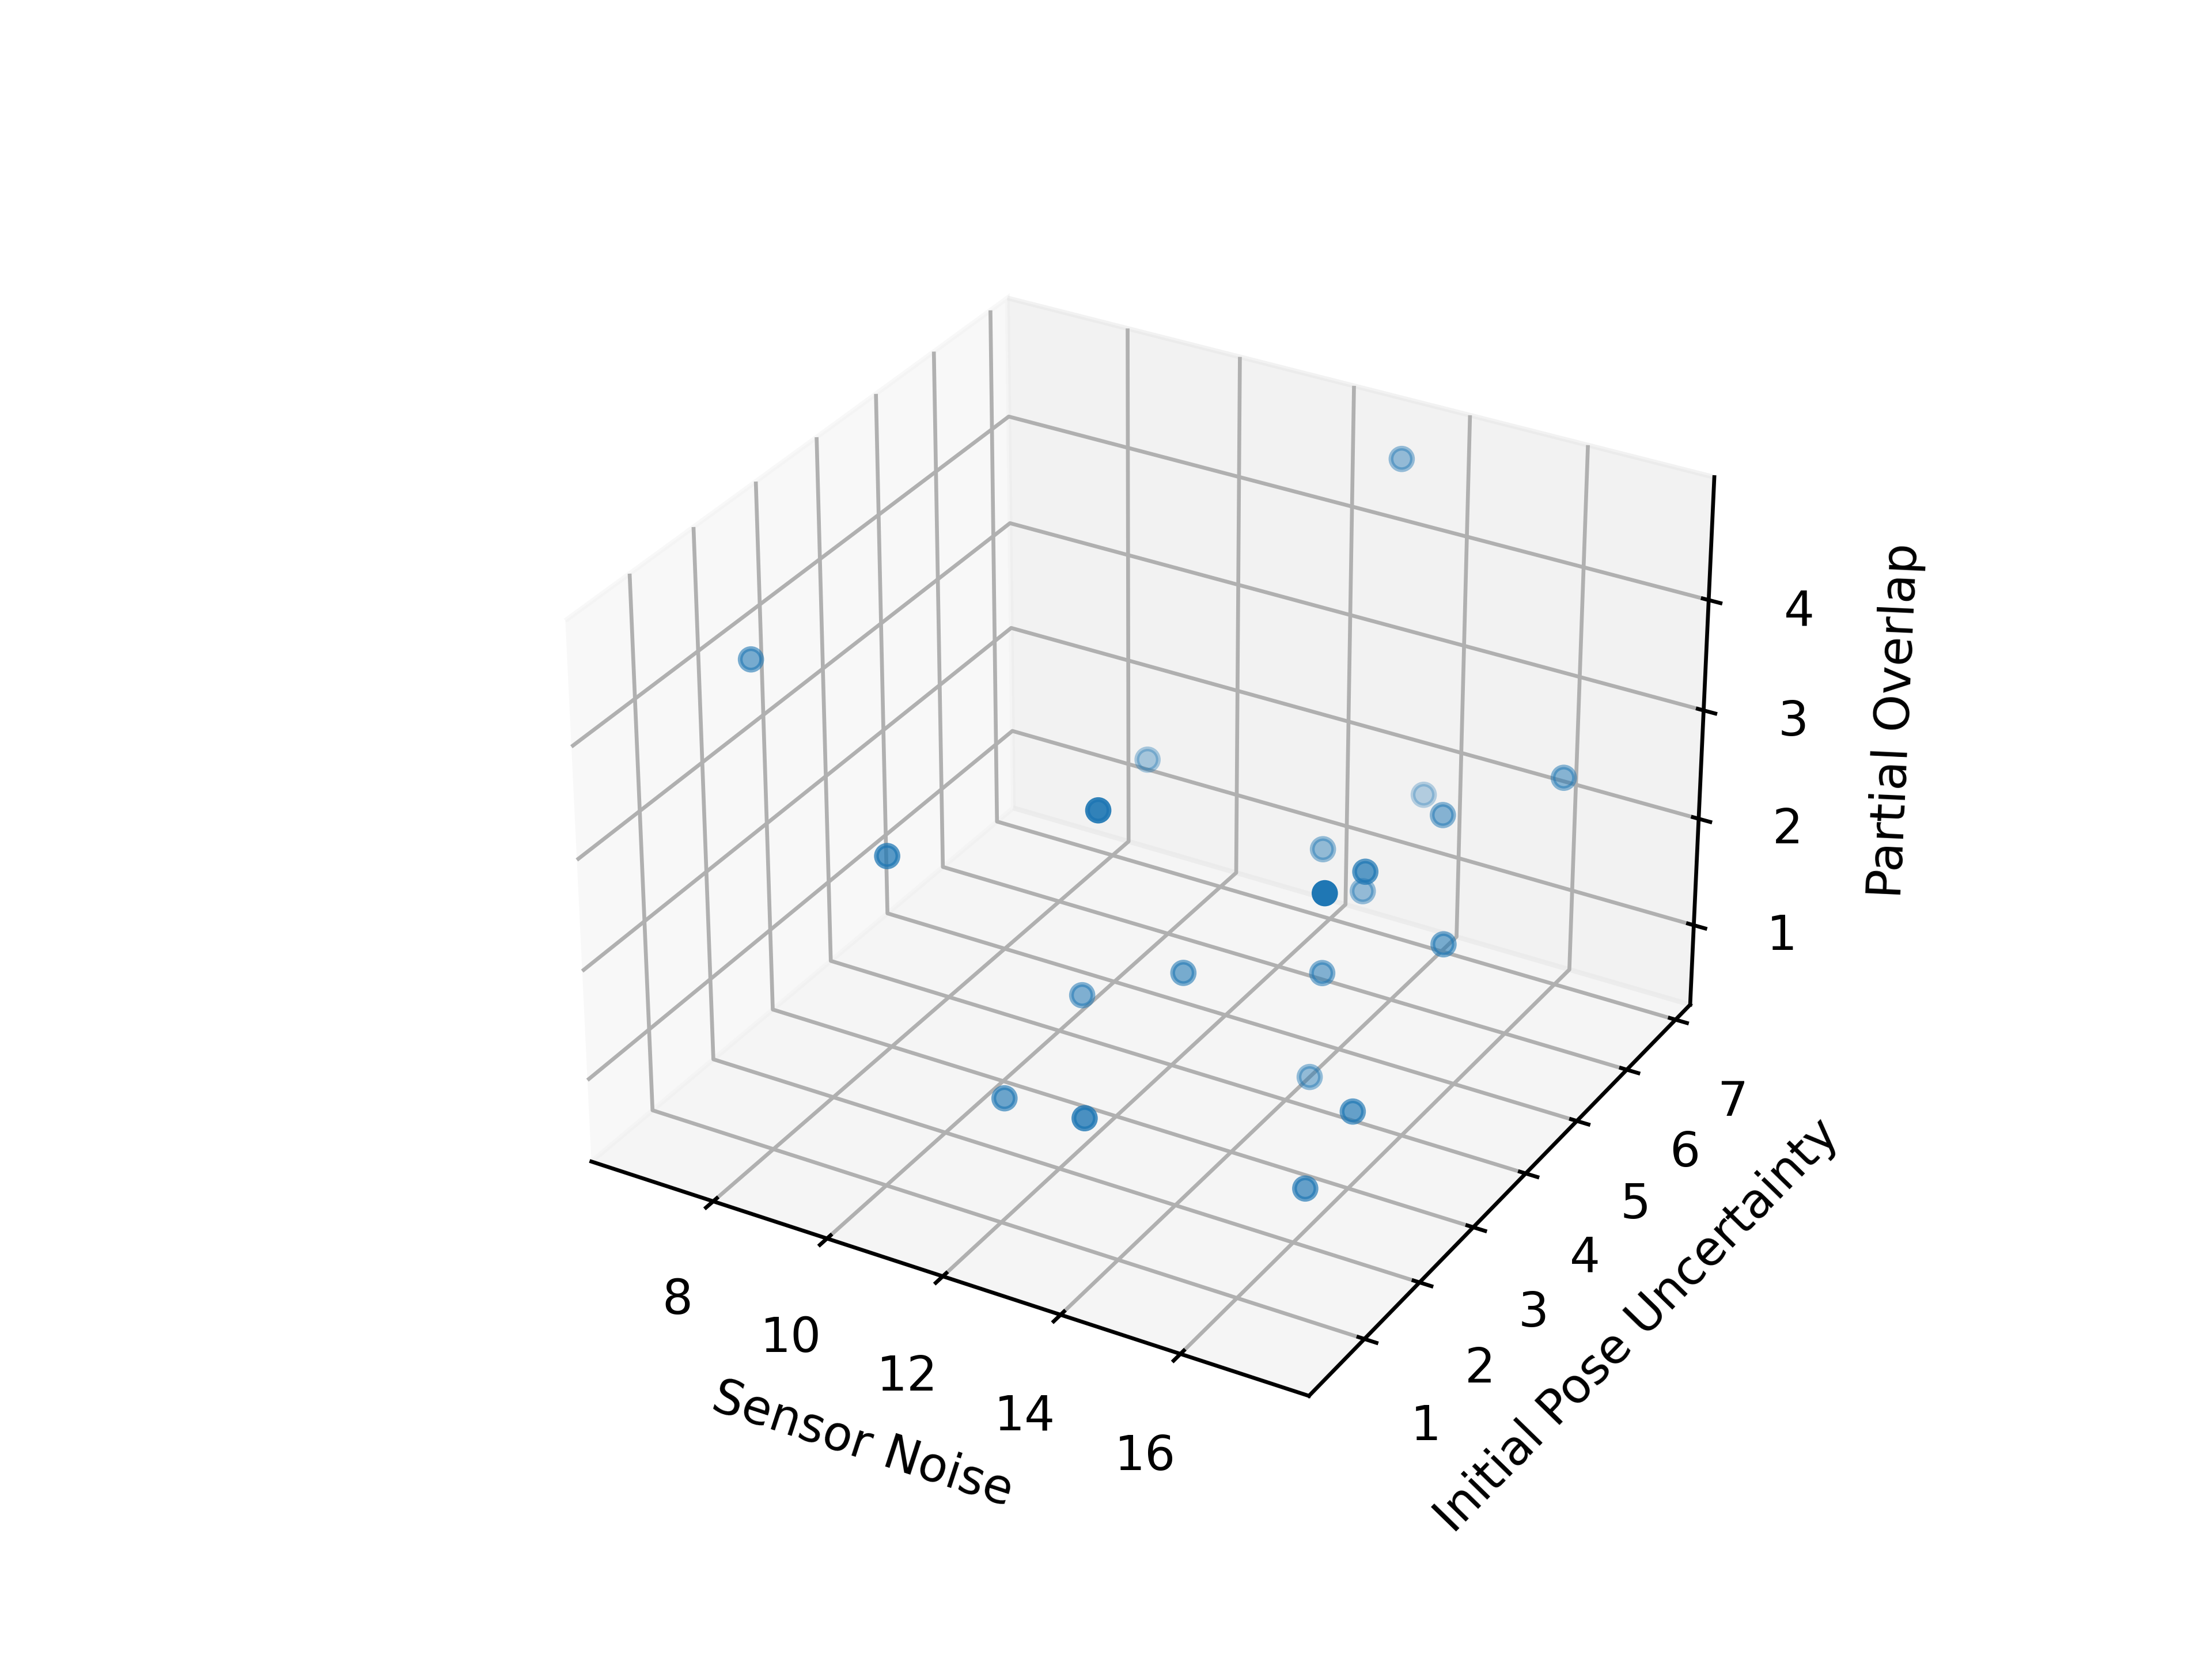}
        \caption{Wood Summer}
    \end{subfigure}
    \hfill
    \begin{subfigure}[b]{0.47\textwidth}
        \includegraphics[width=\linewidth]{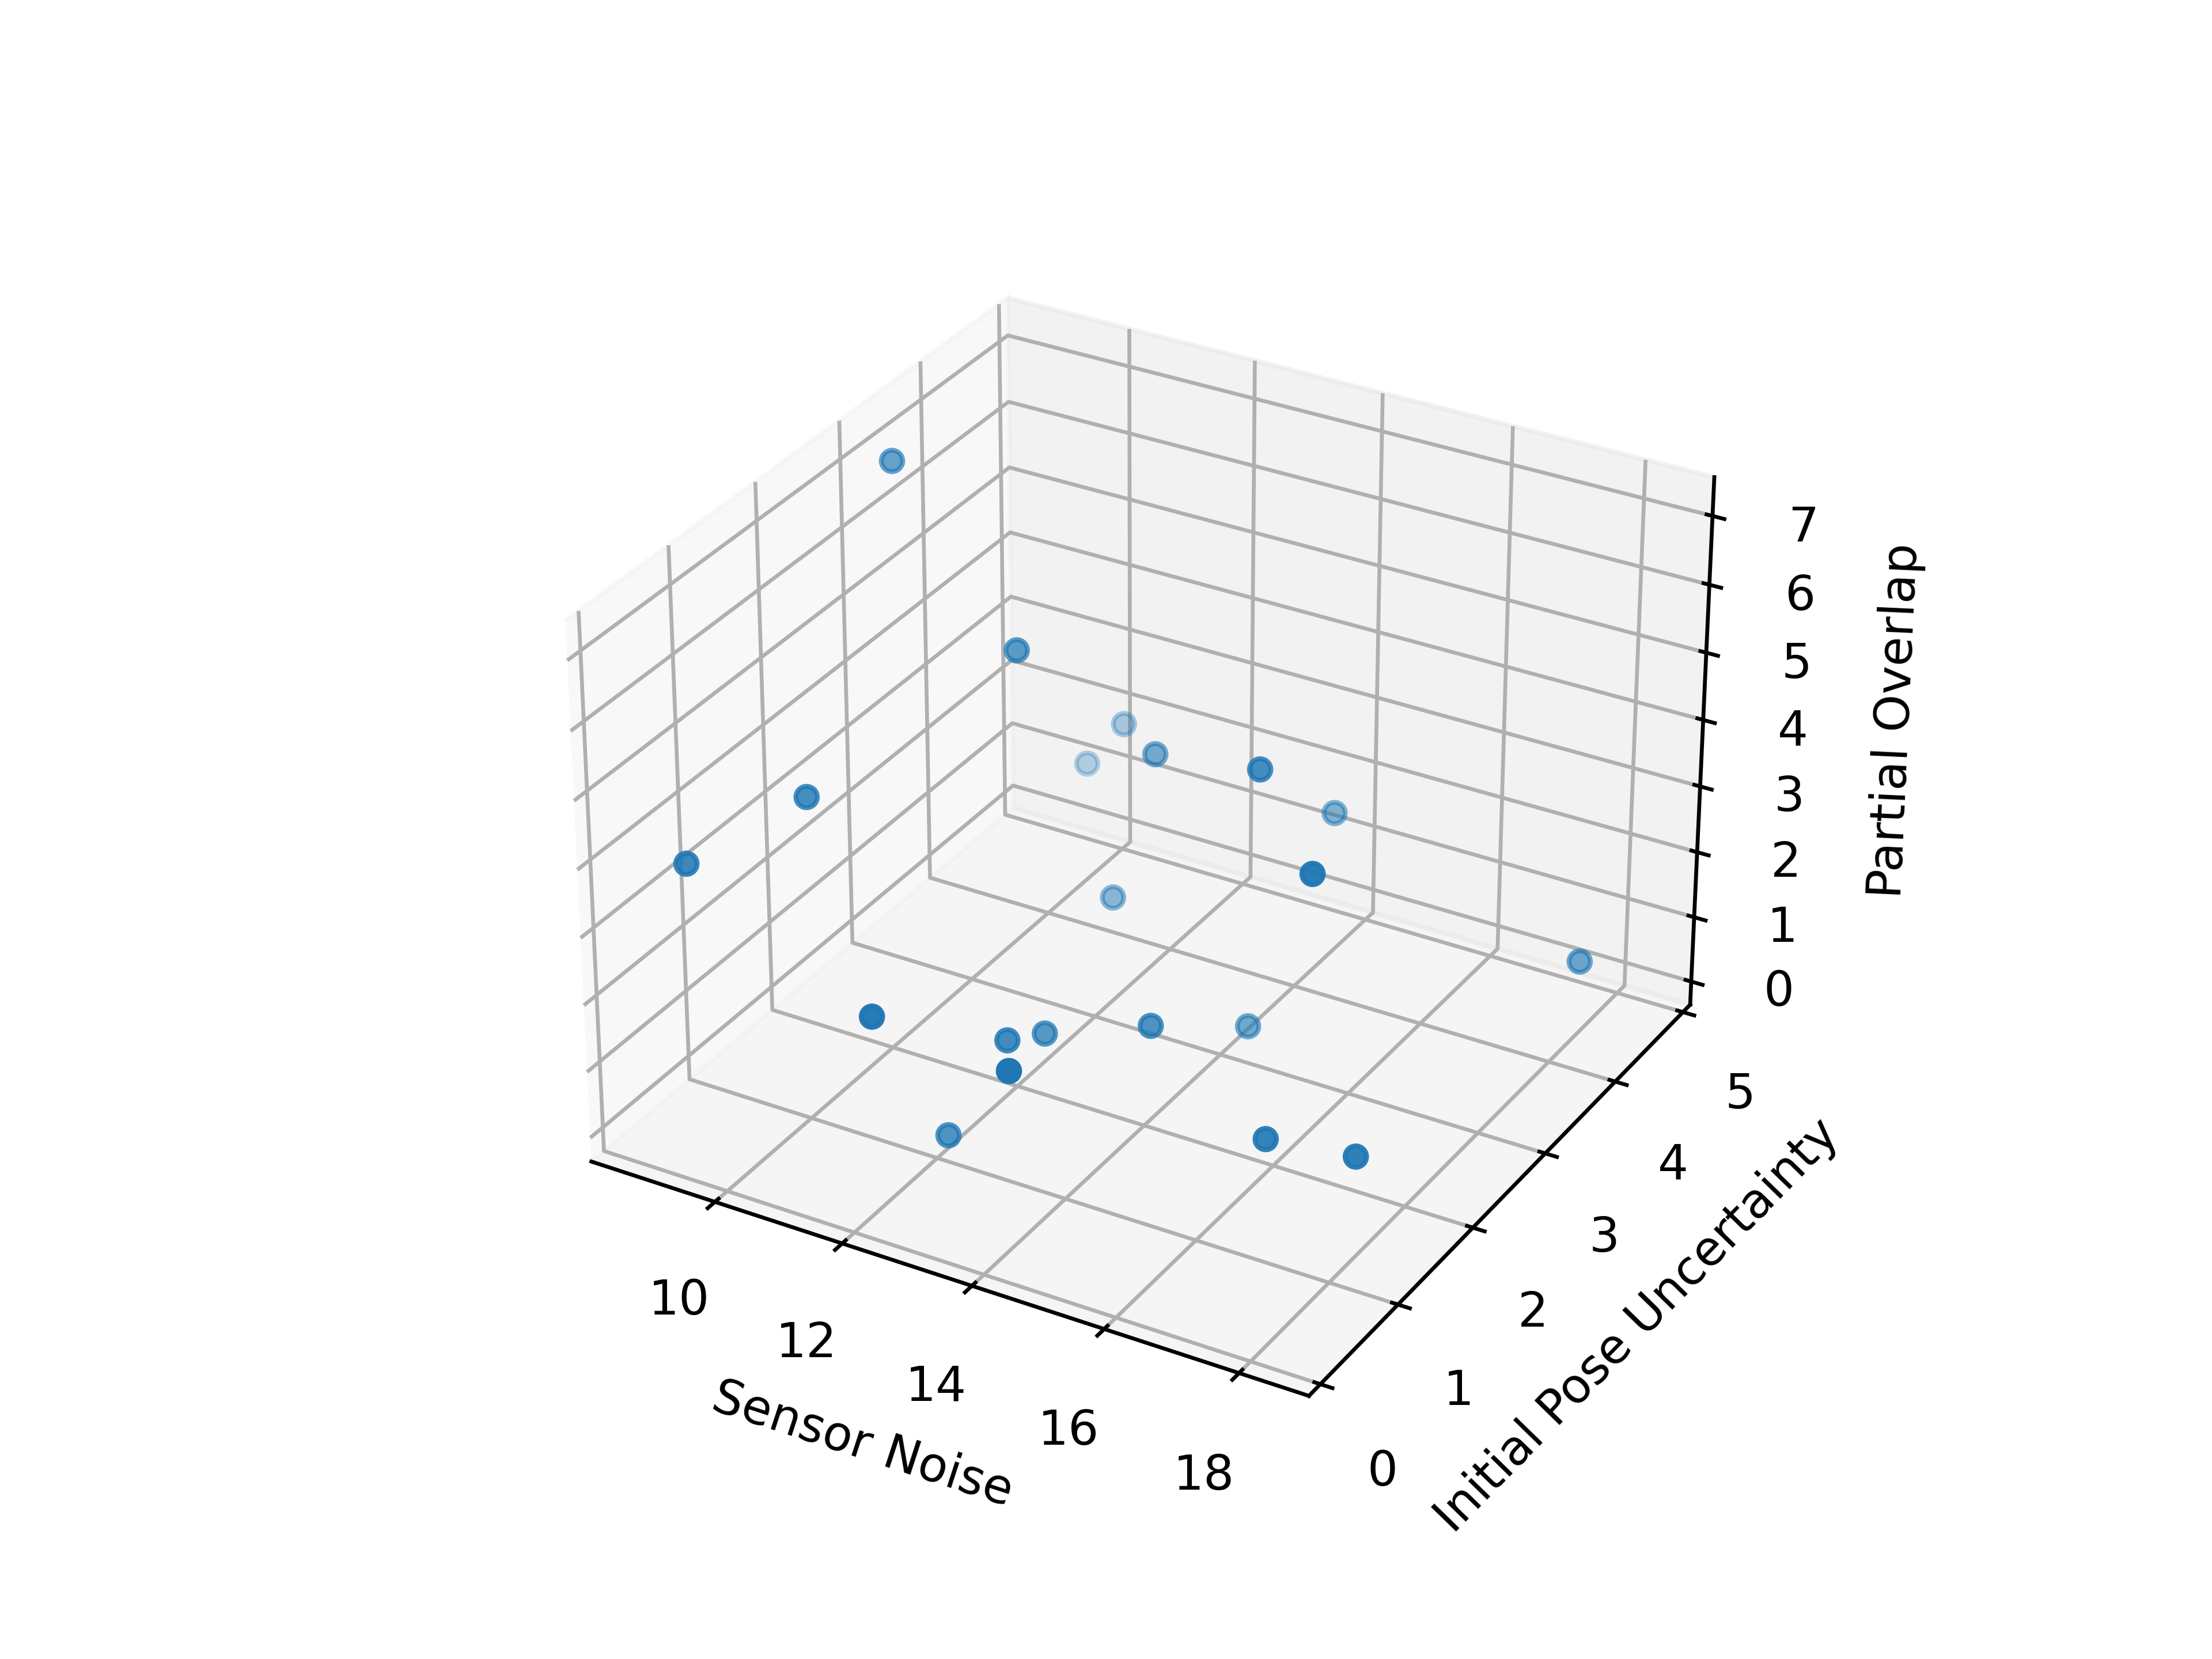}
        \caption{Wood Autumn}
    \end{subfigure}
    \caption{Inlier SHAP values of three uncertainty sources in all sequences.}
    \label{fig:all_seq}
\end{figure}
\clearpage % ends page
\restoregeometry

\section{Caveats}

Granted, kernel SHAP could effectively explain the effect of each uncertainty source for one ICP uncertainty estimate, there exist some \textit{caveats} for the three chosen uncertainty sources and explanation methods.

\begin{itemize}
    \item In the original data, sensor noise is assumed to be zero for unperturbed data, but this may be an oversimplified assumption. In reality, the input point clouds would be subjected to sensor noise and current sensor noise perturbation level should be quantified. To attain the reference value of $0$, they would have to be denoised.
    \item The setting of experiments in this work follows from~\citep{brossard2020new}, where initial poses are sampled around ground truth pose. But in practice, this ground truth pose may not be known, and the initial poses may have to be uniformly sampled from a range obtained from some coarse alignment algorithms.
    \item When overlap ratio is already very small, e.g., around $0.4$, removing even $10\%$ of points in overlapping region may induce unreasonable SHAP values.
    \item Kernel SHAP could identify how important a feature is to the model, but if the model changes, uncertainty has to be recalculated and conclusions of feature importance might differ.
    \item As explanation methods trade interpretability with complexity, they may be able to simplify prediction of one data instance to a linear explanation model, but cannot capture the complexity of the original model. This is an inherent limitation in interpretable explanation models.
\end{itemize}
